# Supplementary material for: Neural Models for Offensive Language Detection
Source: arXiv:2106.14609 source file (2021-05-30)
Supplement: Supplementary file 1 [file appendix.tex]

% !TeX spellcheck = en_US
% !TeX encoding = UTF-8
\chapter{Code}

\chapter{Math}

\chapter{Dataset}
